# Supplementary material for: Benchmarking the accuracy of the separable resolution of the identity approach for correlated methods in the numeric atom-centered orbitals framework
Source: arXiv:2310.11058 ancillary file (2024-01-12)
Supplement: Supplementary file 1 [file Supporting_Information.pdf]

# Supporting Information: Benchmarking the accuracy of the separable resolution of the identity approach for correlated methods in the numeric atom-centered orbitals framework

Francisco A. Delesma[1], Moritz Leucke[2], Dorothea Golze[2], Patrick Rinke[1]

[1] Department of Applied Physics, Aalto University, FI-02150 Espoo, Finland
[2] Faculty for Chemistry and Food Chemistry, Technische Universität Dresden, 01062 Dresden, Germany

January 12, 2024

## S1 Real-space grids for the Def2-TZVP basis

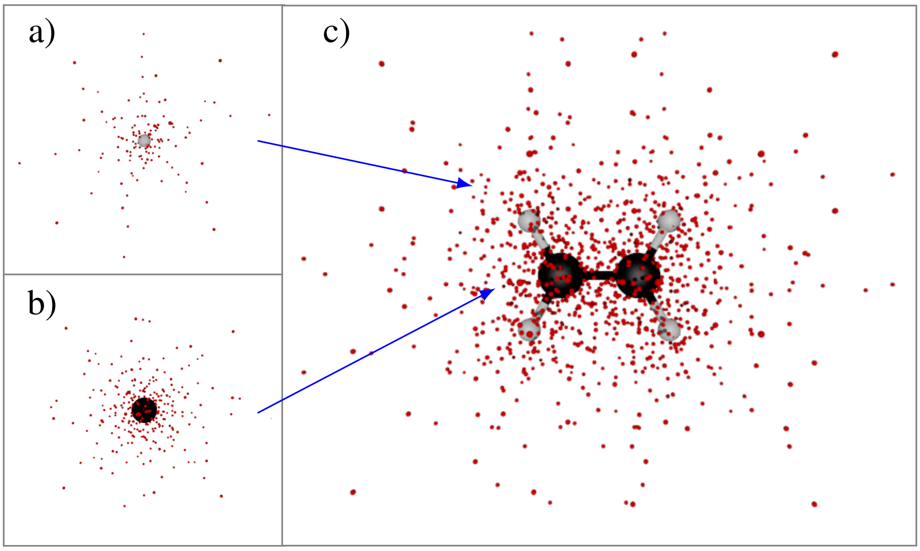


Figure S1: Real space grid $\mathbf{r}_k$ (red dots) for a) the hydrogen atom, b) carbon atom and c) ethylene molecule. The real space grid for a given molecule is constructed by the superposition of the grid of each species. Displayed are the grids for the Def2-TZVP basis set.

## S2 Hartree-Fock and MP2 total and atomization energies employing the Def2-TZVP basis set

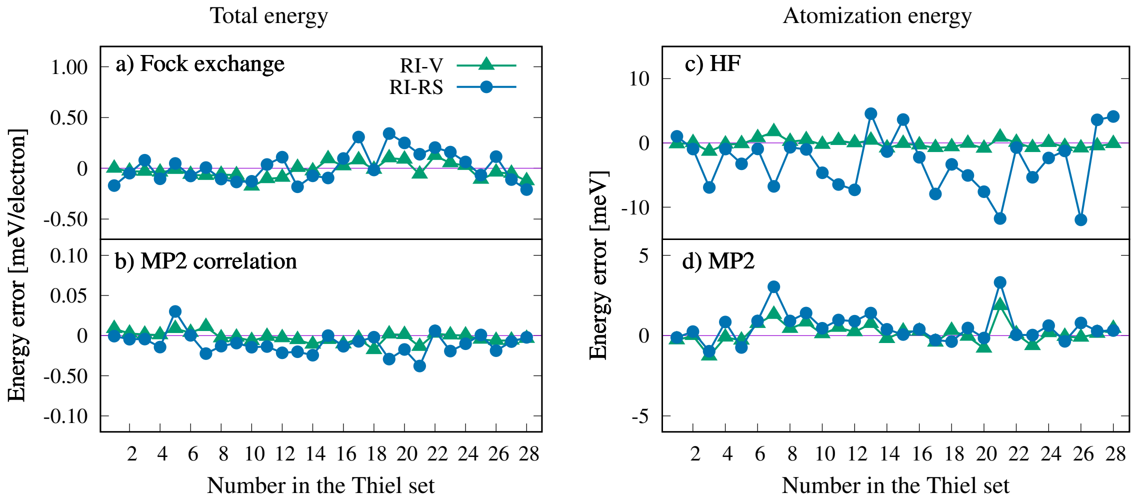


Figure S2: a) Errors of RI-V and RI-RS with respect to the non-RI reference. Total energy errors [meV/electron] for a) HF exchange and b) MP2 correlation energy. Atomization energy errors [meV] for c) HF and d) MP2. The errors are defined as $E^{\text{RI-V/RI-RS}} - E^{\text{non-RI}}$. The Def2-TZVP basis set was used.

## S3 Total, atomization and quasiparticle energies employing the cc-pVTZ basis set

Table S1: Total Hartree-Fock energies in eV

| | Thiel set | no-RI | RI-V | RI-RS |
|---|---|---|---|---|
| 1 | Ethene | -2124.21468977 | -2124.21407633 | -2124.20481330 |
| 2 | Butadiene | -4217.12971069 | -4217.13037169 | -4217.12829002 |
| 3 | Hexatriene | -6310.05377040 | -6310.05315343 | -6310.02943517 |
| 4 | Octatetraene | -8402.97859680 | -8402.97959891 | -8402.95977352 |
| 5 | Cyclopropene | -3152.82929252 | -3152.82935347 | -3152.82543204 |
| 6 | Cyclopentadiene | -5247.89840735 | -5247.89807779 | -5247.88996526 |
| 7 | Norbornadiene | -7339.95333338 | -7339.95305174 | -7339.94389402 |
| 8 | Benzene | -6279.80177691 | -6279.79932961 | -6279.79497851 |
| 9 | Naphthalene | -10434.85385411 | -10434.85008627 | -10434.86362094 |
| 10 | Furan | -6223.38524540 | -6223.38470033 | -6223.38048011 |
| 11 | Pyrrole | -5683.98390856 | -5683.98450613 | -5683.97851582 |
| 12 | Imidazole | -6119.63835932 | -6119.63817904 | -6119.62780116 |
| 13 | Pyridine | -6715.08819452 | -6715.08713158 | -6715.09375347 |
| 14 | Pyrazine | -7150.22296886 | -7150.22242544 | -7150.21959191 |
| 15 | Pyrimidine | -7150.53195527 | -7150.53189942 | -7150.54090530 |
| 16 | Pyridazine | -7149.30528428 | -7149.30521865 | -7149.30556886 |
| 17 | Triazine | -7586.12431207 | -7586.12452658 | -7586.12715983 |

(*Table S1 continues*)

(*Table S1 continued*)

| | Thiel set | no-RI | RI-V | RI-RS |
|---|---|---|---|---|
| 18 | Tetrazine | -8018.73853176 | -8018.73928486 | -8018.73406517 |
| 19 | Formaldehyde | -3099.64022751 | -3099.64007925 | -3099.63817691 |
| 20 | Acetone | -5225.45485219 | -5225.45440296 | -5225.46455226 |
| 21 | Benzoquinone | -10322.87105814 | -10322.86950561 | -10322.85964856 |
| 22 | Formamide | -4598.71090877 | -4598.71117700 | -4598.70633147 |
| 23 | Acetamide | -5661.54093809 | -5661.54088573 | -5661.54191078 |
| 24 | Propanamide | -6724.09502336 | -6724.09529851 | -6724.09892279 |
| 25 | Cytosine | -10687.46871070 | -10687.46866682 | -10687.45256612 |
| 26 | Thymine | -12290.48745532 | -12290.48670069 | -12290.47032134 |
| 27 | Uracil | -11227.84446653 | -11227.84414751 | -11227.82617222 |
| 28 | Adenine | -12644.46333770 | -12644.46295862 | -12644.47212587 |
| | Atom | | | |
| 1 | Hydrogen | -13.60051695 | -13.60051610 | -13.60051610 |
| 2 | Carbon | -1025.63978117 | -1025.63980123 | -1025.64059635 |
| 3 | Nitrogen | -1480.31798943 | -1480.31802735 | -1480.31827007 |
| 4 | Oxygen | -2035.73147450 | -2035.73146634 | -2035.73181819 |

Table S2: Hartree-Fock exchange energies in eV

| | Thiel set | no-RI | RI-V | RI-RS |
|---|---|---|---|---|
| 1 | Ethene | -319.55713413 | -319.55718104 | -319.54793684 |
| 2 | Butadiene | -620.93812416 | -620.93895089 | -620.93458450 |
| 3 | Hexatriene | -922.33296692 | -922.33402217 | -922.30458764 |
| 4 | Octatetraene | -1223.72167581 | -1223.72369952 | -1223.69733642 |
| 5 | Cyclopropene | -460.47217945 | -460.47252677 | -460.46835578 |
| 6 | Cyclopentadiene | -763.44055083 | -763.44250535 | -763.43592180 |
| 7 | Norbornadiene | -1066.26459776 | -1066.26791603 | -1066.26340694 |
| 8 | Benzene | -904.66171486 | -904.66367200 | -904.65397966 |
| 9 | Naphthalene | -1489.55902782 | -1489.56276059 | -1489.57247081 |
| 10 | Furan | -826.85994223 | -826.86623201 | -826.85548648 |
| 11 | Pyrrole | -792.94705463 | -792.95052594 | -792.94217384 |
| 12 | Imidazole | -821.73063497 | -821.73353947 | -821.71787850 |
| 13 | Pyridine | -933.33007995 | -933.32912336 | -933.33209988 |
| 14 | Pyrazine | -961.60193472 | -961.60274779 | -961.60232830 |
| 15 | Pyrimidine | -962.26494117 | -962.26025098 | -962.26513597 |
| 16 | Pyridazine | -960.53809932 | -960.53708099 | -960.53774637 |
| 17 | Triazine | -991.41246293 | -991.40844207 | -991.41239033 |
| 18 | Tetrazine | -1016.07434899 | -1016.07492652 | -1016.07340733 |
| 19 | Formaldehyde | -383.02258307 | -383.02105504 | -383.01683018 |
| 20 | Acetone | -705.46337097 | -705.46091486 | -705.47353969 |
| 21 | Benzoquinone | -1332.35800404 | -1332.36173822 | -1332.34458294 |
| 22 | Formamide | -574.28692740 | -574.28403988 | -574.27664274 |
| 23 | Acetamide | -735.51992088 | -735.51848376 | -735.51842667 |
| 24 | Propanamide | -896.65069936 | -896.64980707 | -896.65556470 |
| 25 | Cytosine | -1379.10746927 | -1379.11369453 | -1379.09174022 |
| 26 | Thymine | -1574.73578430 | -1574.73864226 | -1574.71962161 |
| 27 | Uracil | -1413.51857191 | -1413.52476178 | -1413.50501973 |
| 28 | Adenine | -1655.98544570 | -1655.99356460 | -1656.00972609 |
| | Atom | | | |
| 1 | Hydrogen | -8.50448457 | 8.50448527 | -8.50448494 |
| 2 | Carbon | -138.15858759 | 138.15917461 | -138.16016701 |
| 3 | Nitrogen | -179.81436104 | 179.81461047 | -179.81486601 |
| 4 | Oxygen | -223.69067209 | 223.69072606 | -223.69098426 |

Table S3: MP2 and CCSD correlation energies in eV

| | | MP2 | | | CCSD | |
|---|---|---|---|---|---|---|
| | Thiel set | no-RI | RI-V | RI-RS | RI-V | RI-RS |
| 1 | Ethene | -9.96527457 | -9.96521554 | -9.96574426 | -10.65746083 | -10.65771622 |
| 2 | Butadiene | -19.39699287 | -19.39697230 | -19.39678753 | -20.41786654 | -20.41784089 |
| 3 | Hexatriene | -28.87996837 | -28.87994986 | -28.88179017 | -30.19787644 | -30.19920261 |
| 4 | Octatetraene | -38.38260273 | -38.38262003 | -38.38200750 | -39.98392906 | -39.98359704 |
| 5 | Cyclopropene | -14.51781283 | -14.51762411 | -14.51741731 | -15.14217908 | -15.14195212 |
| 6 | Cyclopentadiene | -24.04265993 | -24.04260735 | -24.04238639 | -24.93704739 | -24.93695440 |
| 7 | Norbornadiene | -34.06584288 | -34.06534231 | -34.06511591 | -35.13831493 | -35.13821169 |
| 8 | Benzene | -28.38878091 | -28.38901240 | -28.38743795 | -29.12001675 | -29.11943067 |
| 9 | Naphthalene | -46.99721485 | -46.99781620 | -46.99275298 | -47.77021743 | -47.76788398 |
| 10 | Furan | -25.73036855 | -25.73068681 | -25.73189908 | -26.15334132 | -26.15408619 |
| 11 | Pyrrole | -25.20755752 | -25.20764128 | -25.20674711 | -25.69952682 | -25.69913711 |
| 12 | Imidazole | -26.08471764 | -26.08484379 | -26.08438093 | -26.38359577 | -26.38328544 |
| 13 | Pyridine | -29.28981926 | -29.29009318 | -29.28874731 | -29.83027829 | -29.82942132 |
| 14 | Pyrazine | -30.23551943 | -30.23596853 | -30.23658541 | -30.55764510 | -30.55833331 |
| 15 | Pyrimidine | -30.08961720 | -30.08984693 | -30.08853670 | -30.46940302 | -30.46857955 |
| 16 | Pyridazine | -30.34351635 | -30.34399364 | -30.34443936 | -30.64601331 | -30.64700807 |
| 17 | Triazine | -30.81090679 | -30.81106182 | -30.81058018 | -31.05219102 | -31.05212119 |
| 18 | Tetrazine | -32.27851549 | -32.27918268 | -32.28121782 | -32.15840278 | -32.16014686 |
| 19 | Formaldehyde | -11.56908183 | -11.56901645 | -11.56949700 | -11.84186362 | -11.84199930 |
| 20 | Acetone | -21.83320621 | -21.83321408 | -21.83457982 | -22.67338166 | -22.67429286 |
| 21 | Benzoquinone | -40.71075762 | -40.71146093 | -40.71347512 | -41.23468661 | -41.23599246 |
| 22 | Formamide | -17.65307350 | -17.65295494 | -17.65279929 | -17.93551377 | -17.93526625 |
| 23 | Acetamide | -22.77001029 | -22.76997334 | -22.77035321 | -23.35126281 | -23.35150563 |
| 24 | Propanamide | -27.96020938 | -27.96020615 | -27.96140209 | -28.83065285 | -28.83165297 |
| 25 | Cytosine | -42.79398232 | -42.79427336 | -42.79395254 | -43.20002457 | -43.19939658 |
| 26 | Thymine | -48.65134658 | -48.65171735 | -48.65314241 | -49.17241001 | -49.17299350 |
| 27 | Uracil | -43.37033988 | -43.37061103 | -43.36936965 | -43.64298177 | -43.64176514 |
| 28 | Adenine | -52.31876349 | -52.31903129 | -52.31736513 | -52.40956356 | -52.40881254 |
| | Atom | | | | | |
| 1 | Carbon | -2.05910988 | -2.05907485 | -2.05911567 | -2.60630528 | -2.60635187 |
| 2 | Nitrogen | -2.88780076 | -2.88772763 | -2.88777253 | -3.31478575 | -3.31483550 |
| 3 | Oxygen | -4.19641186 | -4.19610080 | -4.19612093 | -4.63067122 | -4.63068851 |

Table S4: Total PBE, PBE exchange-correlation and Hartree-Fock exchange energies in eV

| | Thiel set | PBE | $E_{xc}^{PBE}$ | $E_x^{HF}$ |
|---|---|---|---|---|
| 1 | Ethene | -2136.07756777 | -331.17353174 | -318.83601675 |
| 2 | Butadiene | -4240.26522356 | -643.49805123 | -619.33905923 |
| 3 | Hexatriene | -6344.50764741 | -955.88320563 | -919.84413115 |
| 4 | Octatetraene | -8448.77591669 | -1268.28417221 | -1220.34049613 |
| 5 | Cyclopropene | -3170.17279419 | -477.44967754 | -459.44528394 |
| 6 | Cyclopentadiene | -5276.43390640 | -791.02384262 | -761.28213547 |
| 7 | Norbornadiene | -7379.91376764 | -1104.49109761 | -1062.83878615 |
| 8 | Benzene | -6313.43920021 | -937.70737838 | -902.73781124 |
| 9 | Naphthalene | -10490.33399263 | -1543.98254159 | -1486.23115690 |
| 10 | Furan | -6253.94401258 | -856.34014020 | -824.49163197 |
| 11 | Pyrrole | -5713.79333572 | -822.14523842 | -791.19314674 |
| 12 | Imidazole | -6150.50670004 | -851.91703618 | -819.80791287 |
| 13 | Pyridine | -6749.81509774 | -967.40707192 | -931.26256652 |
| 14 | Pyrazine | -7186.10120437 | -996.92952313 | -959.57240706 |
| 15 | Pyrimidine | -7186.26805965 | -997.16698759 | -959.91252179 |
| 16 | Pyridazine | -7185.36463899 | -996.11713358 | -958.56799278 |
| 17 | Triazine | -7622.78984574 | -1026.97603040 | -988.68164842 |
| 18 | Tetrazine | -8057.20126266 | -1054.27637451 | -1014.18784150 |
| 19 | Formaldehyde | -3113.35766279 | -395.99572941 | -381.67172672 |
| 20 | Acetone | -5251.30351184 | -729.72654343 | -702.71550926 |
| 21 | Benzoquinone | -10371.47414679 | -1378.86577802 | -1327.82329206 |
| 22 | Formamide | -4619.68726740 | -594.02524567 | -572.05187924 |
| 23 | Acetamide | -5688.51229827 | -760.92990343 | -732.72525669 |
| 24 | Propanamide | -6757.10335473 | -927.69299377 | -893.19477974 |
| 25 | Cytosine | -10738.43771236 | -1427.77590372 | -1374.33115462 |
| 26 | Thymine | -12348.28361919 | -1629.48948273 | -1568.84060679 |
| 27 | Uracil | -11279.53927053 | -1462.60944588 | -1408.31916361 |
| 28 | Adenine | -12706.41108505 | -1715.98121981 | -1651.27165885 |
| | Atom | | | |
| 1 | Hydrogen | -13.59533371 | -8.39521190 | -8.38818294 |
| 2 | Carbon | -1028.45223071 | -140.40501311 | -137.48132382 |
| 3 | Nitrogen | -1483.82802060 | -182.63308085 | -179.01485296 |
| 4 | Oxygen | -2040.98751029 | -228.10671012 | -222.69958017 |

Table S5: RPA, SOSEX and rSE correlation energies in eV

| | | RPA | | SOSEX | | rSE | |
|---|---|---|---|---|---|---|---|
| | Thiel set | RI-V | RI-RS | RI-V | RI-RS | RI-V | RI-RS |
| 1 | Ethene | -17.17466358 | -17.17464908 | 6.73103791 | 6.73104132 | -0.41347602 | -0.41332954 |
| 2 | Butadiene | -32.62006299 | -32.62016296 | 12.43358075 | 12.43362018 | -0.86729579 | -0.86777945 |
| 3 | Hexatriene | -48.10186089 | -48.10260288 | 18.11732123 | 18.11757129 | -1.32063578 | -1.32118273 |
| 4 | Octatetraene | -63.59402834 | -63.59344409 | 23.78830839 | 23.78806010 | -1.77037843 | -1.77117111 |
| 5 | Cyclopropene | -23.99540009 | -23.99488993 | 9.09805043 | 9.09807523 | -0.58189132 | -0.58127903 |
| 6 | Cyclopentadiene | -39.41479473 | -39.41390799 | 14.62907342 | 14.62883737 | -1.01507040 | -1.01448032 |
| 7 | Norbornadiene | -55.35646239 | -55.35585227 | 20.42830453 | 20.42822597 | -1.42790452 | -1.42706077 |
| 8 | Benzene | -45.84772957 | -45.84669715 | 16.76358411 | 16.76364601 | -1.15852699 | -1.15786677 |
| 9 | Naphthalene | -74.89622588 | -74.89309465 | 26.99306739 | 26.99232033 | -1.95424288 | -1.95460073 |
| 10 | Furan | -40.62012096 | -40.62060542 | 14.67659844 | 14.67685053 | -1.10631216 | -1.10555085 |
| 11 | Pyrrole | -40.08242965 | -40.08082522 | 14.56536325 | 14.56486431 | -0.98982449 | -0.98862115 |
| 12 | Imidazole | -40.86022371 | -40.85898915 | 14.68652485 | 14.68607350 | -1.06846598 | -1.06833375 |
| 13 | Pyridine | -46.67543470 | -46.67506793 | 16.91520171 | 16.91523434 | -1.22955115 | -1.23060833 |
| 14 | Pyrazine | -47.49000439 | -47.49128319 | 17.06157392 | 17.06198821 | -1.28671341 | -1.28661193 |
| 15 | Pyrimidine | -47.41935974 | -47.41906105 | 17.03238499 | 17.03227120 | -1.30817900 | -1.30955982 |
| 16 | Pyridazine | -47.64558635 | -47.64663045 | 17.12968428 | 17.12978743 | -1.29363476 | -1.29388023 |
| 17 | Triazine | -48.09672310 | -48.09782286 | 17.12467911 | 17.12507567 | -1.39241394 | -1.39359182 |
| 18 | Tetrazine | -49.42588106 | -49.42814836 | 17.49692523 | 17.49714872 | -1.41426871 | -1.41572653 |
| 19 | Formaldehyde | -18.41434441 | -18.41453097 | 6.88437594 | 6.88420490 | -0.54178040 | -0.54208662 |
| 20 | Acetone | -35.73050617 | -35.73320400 | 13.34745701 | 13.34841338 | -1.00000253 | -1.00026681 |
| 21 | Benzoquinone | -64.06707024 | -64.06872068 | 23.10710542 | 23.10768885 | -2.06784432 | -2.06834432 |
| 22 | Formamide | -27.76888757 | -27.76841720 | 10.09623549 | 10.09581874 | -0.85561949 | -0.85592720 |
| 23 | Acetamide | -36.39430246 | -36.39491600 | 13.33485675 | 13.33492786 | -1.05816415 | -1.05829865 |
| 24 | Propanamide | -45.15236572 | -45.15403219 | 16.63972282 | 16.64003752 | -1.27597470 | -1.27610499 |
| 25 | Cytosine | -66.84227956 | -66.84031683 | 23.74537259 | 23.74450993 | -2.08724024 | -2.08708777 |
| 26 | Thymine | -76.08201399 | -76.08303453 | 27.10324086 | 27.10324342 | -2.41790276 | -2.41884726 |
| 27 | Uracil | -67.27338045 | -67.27185687 | 23.81102069 | 23.81054373 | -2.20575621 | -2.20667344 |
| 28 | Adenine | -80.75025593 | -80.74965894 | 28.39522130 | 28.39445180 | -2.32781078 | -2.32918914 |
| | Atom | | | | | | |
| 1 | Hydrogen | -0.49657859 | -0.49657858 | 0.49657859 | 0.49657858 | -0.00925482 | -0.00925482 |
| 2 | Carbon | -4.96821779 | -4.96826093 | 2.59328287 | 2.59326992 | -0.08895848 | -0.08896999 |
| 3 | Nitrogen | -5.75688963 | -5.75692429 | 2.70388350 | 2.70386502 | -0.08834742 | -0.08834763 |
| 4 | Oxygen | -7.71801862 | -7.71802786 | 3.40743257 | 3.40741553 | -0.12647607 | -0.12646869 |

Table S6: Hartree-Fock and MP2 atomization energies in eV

| | | Hartree-Fock | | | MP2 | | |
|---|---|---|---|---|---|---|---|
| | Thiel set | no-RI | RI-V | RI-RS | no-RI | RI-V | RI-RS |
| 1 | Ethene | 18.53305962 | 18.53240947 | 18.52155621 | 24.38011443 | 24.37947531 | 24.37992239 |
| 2 | Butadiene | 32.96748430 | 32.96807017 | 32.96280803 | 44.12803765 | 44.12874306 | 44.12839503 |
| 3 | Hexatriene | 47.41094778 | 47.41021725 | 47.38172829 | 63.93625687 | 63.93571800 | 63.93731340 |
| 4 | Octatetraene | 61.85517794 | 61.85602807 | 61.82984174 | 83.76490163 | 83.76604928 | 83.76511022 |
| 5 | Cyclopropene | 21.50788121 | 21.50788538 | 21.50157860 | 29.84836440 | 29.84828494 | 29.84795568 |
| 6 | Cyclopentadiene | 38.09639980 | 38.09597504 | 38.08388692 | 51.84351032 | 51.84320812 | 51.84278308 |
| 7 | Norbornadiene | 51.67072959 | 51.67031433 | 51.65559079 | 71.32280331 | 71.32213267 | 71.32162055 |
| 8 | Benzene | 44.35998818 | 44.35742563 | 44.34830383 | 60.39410982 | 60.39198892 | 60.39016957 |
| 9 | Naphthalene | 69.65190681 | 69.64794517 | 69.65352867 | 96.05802287 | 96.05501284 | 96.04954145 |
| 10 | Furan | 30.69257842 | 30.69196466 | 30.68421214 | 43.99009559 | 43.99025126 | 43.99128013 |
| 11 | Pyrrole | 46.70472665 | 46.70520946 | 46.69579596 | 60.78804389 | 60.78882370 | 60.78772136 |
| 12 | Imidazole | 27.68096915 | 27.68065625 | 27.66740758 | 41.81275563 | 41.81282022 | 41.81214511 |
| 13 | Pyridine | 38.56871449 | 38.56751758 | 38.56992116 | 54.67518359 | 54.67450887 | 54.67291401 |
| 14 | Pyrazine | 32.62579752 | 32.62510142 | 32.61860198 | 48.84927592 | 48.84931527 | 48.84967908 |
| 15 | Pyrimidine | 32.93478393 | 32.93457541 | 32.93991537 | 49.01236009 | 49.01266766 | 49.01110436 |
| 16 | Pyridazine | 31.70811295 | 31.70789463 | 31.70457892 | 48.03958826 | 48.04013359 | 48.04032625 |
| 17 | Triazine | 27.44944942 | 27.44949255 | 27.44901227 | 43.41962429 | 43.42014691 | 43.41940812 |
| 18 | Tetrazine | 18.98597781 | 18.98654081 | 18.97875999 | 35.59507050 | 35.59666325 | 35.59843716 |
| 19 | Formaldehyde | 11.06793794 | 11.06777948 | 11.06473017 | 16.38149803 | 16.38162028 | 16.38203988 |
| 20 | Acetone | 31.20093248 | 31.20043632 | 31.20784843 | 42.66039719 | 42.66032505 | 42.66154820 |
| 21 | Benzoquinone | 43.16735433 | 43.16570114 | 43.15036970 | 63.13062894 | 63.13051136 | 63.13224037 |
| 22 | Formamide | 16.22011282 | 16.22033378 | 16.21409856 | 24.72986382 | 24.73038543 | 24.73012393 |
| 23 | Acetamide | 26.20932707 | 26.20920907 | 26.20804932 | 37.77690498 | 37.77720428 | 37.77743748 |
| 24 | Propanamide | 35.92259727 | 35.92278843 | 35.92343279 | 50.62126438 | 50.62194159 | 50.62295004 |
| 25 | Cytosine | 40.22155849 | 40.22133301 | 40.20097182 | 61.91928715 | 61.92002326 | 61.91938434 |
| 26 | Thymine | 48.58651992 | 48.58561056 | 48.56406649 | 72.77389185 | 72.77429678 | 72.77538768 |
| 27 | Uracil | 38.78434620 | 38.78389081 | 38.76154591 | 59.74982132 | 59.75054556 | 59.74901084 |
| 28 | Adenine | 46.67189995 | 46.67123523 | 46.67521327 | 74.25611025 | 74.25625408 | 74.25415935 |

Table S7: CCSD, RPA and rPT2 atomization energies in eV

| | | CCSD | | RPA | | rPT2 | |
|---|---|---|---|---|---|---|---|
| | Thiel set | RI-V | RI-RS | RI-V | RI-RS | RI-V | RI-RS |
| 1 | Ethene | 23.97725975 | 23.97742194 | 23.58166416 | 23.58156342 | 24.22204613 | 24.22176104 |
| 2 | Butadiene | 42.96071561 | 42.96050356 | 42.22995683 | 42.22988430 | 43.60491205 | 43.60508589 |
| 3 | Hexatriene | 61.97026204 | 61.97130861 | 60.91081059 | 60.91129381 | 63.03866164 | 63.03855293 |
| 4 | Octatetraene | 80.98951493 | 80.98881011 | 79.60336021 | 79.60243094 | 82.49326308 | 82.49376324 |
| 5 | Cyclopropene | 28.83114864 | 28.83078188 | 28.33398906 | 28.33334952 | 29.28009820 | 29.27925831 |
| 6 | Cyclopentadiene | 50.00149605 | 50.00117006 | 49.11389686 | 49.11279448 | 50.94545842 | 50.94476639 |
| 7 | Norbornadiene | 68.56449233 | 68.56406289 | 67.46153593 | 67.46062391 | 69.88999680 | 69.88875842 |
| 8 | Benzene | 57.83961073 | 57.83874506 | 56.82750611 | 56.82621491 | 59.17233794 | 59.17121023 |
| 9 | Naphthalene | 91.35510984 | 91.35231040 | 89.83217295 | 89.82861040 | 93.73518250 | 93.73561141 |
| 10 | Furan | 41.78941366 | 41.78995485 | 41.09065519 | 41.09095789 | 42.76791805 | 42.76661535 |
| 11 | Pyrrole | 58.66472942 | 58.66410357 | 58.63042032 | 58.62860871 | 59.63701028 | 59.63598212 |
| 12 | Imidazole | 39.61576469 | 39.61521506 | 39.49462414 | 39.49319088 | 40.56990568 | 40.56991530 |
| 13 | Pyridine | 52.05148374 | 52.05034402 | 51.47113092 | 51.47051384 | 53.35925724 | 53.35989044 |
| 14 | Pyrazine | 46.12795392 | 46.12835622 | 45.97415698 | 45.97519394 | 47.39696127 | 47.39606840 |
| 15 | Pyrimidine | 46.34918582 | 46.34807645 | 46.17301789 | 46.17247736 | 47.64647670 | 47.64759421 |
| 16 | Pyridazine | 45.29911533 | 45.29982420 | 45.20114883 | 45.20195109 | 46.56276412 | 46.56252933 |
| 17 | Triazine | 40.73841048 | 40.73805161 | 40.94721157 | 40.94807796 | 42.03649912 | 42.03691759 |
| 18 | Tetrazine | 32.67319003 | 32.67464191 | 33.50859583 | 33.51063823 | 33.87137995 | 33.87226568 |
| 19 | Formaldehyde | 15.67266661 | 15.67273840 | 15.48307931 | 15.48321351 | 15.90041220 | 15.90080297 |
| 20 | Acetone | 41.42423094 | 41.42498505 | 40.72500643 | 40.72756566 | 42.09542424 | 42.09451045 |
| 21 | Benzoquinone | 59.50121367 | 59.50220534 | 58.58184300 | 58.58321616 | 61.07973632 | 61.07920949 |
| 22 | Formamide | 23.60408530 | 23.60372415 | 23.46629764 | 23.46574026 | 24.08846992 | 24.08905453 |
| 23 | Acetamide | 36.40240436 | 36.40248694 | 36.01893699 | 36.01942040 | 37.08400460 | 37.08386054 |
| 24 | Propanamide | 48.98906848 | 48.98986176 | 48.40796332 | 48.40945654 | 49.86494734 | 49.86448788 |
| 25 | Cytosine | 58.42110800 | 58.42012707 | 58.22534233 | 58.22309386 | 60.14869114 | 60.14895197 |
| 26 | Thymine | 68.83558025 | 68.83579666 | 68.19349723 | 68.19421432 | 70.74670886 | 70.74716829 |
| 27 | Uracil | 56.11073753 | 56.10920043 | 55.66563480 | 55.66385090 | 57.81994812 | 57.82092741 |
| 28 | Adenine | 69.47534365 | 69.47411089 | 69.71015454 | 69.70916860 | 71.67866522 | 71.68020833 |

Table S8: HOMO quasiparticle energies in eV

| | Thiel set | RI-V | RI-RS |
|---|---|---|---|
| 1 | Ethene | -10.20150 | -10.19690 |
| 2 | Butadiene | -8.60750 | -8.60810 |
| 3 | Hexatriene | -7.72700 | -7.72590 |
| 4 | Octatetraene | -7.14930 | -7.15050 |
| 5 | Cyclopropene | -9.56940 | -9.56950 |
| 6 | Cyclopentadiene | -8.11900 | -8.11760 |
| 7 | Norbornadiene | -8.21750 | -8.21640 |
| 8 | Benzene | -8.83410 | -8.83540 |
| 9 | Naphthalene | -7.61800 | -7.62010 |
| 10 | Furan | -8.46200 | -8.46360 |
| 11 | Pyrrole | -7.83550 | -7.83630 |
| 12 | Imidazole | -8.48780 | -8.48700 |
| 13 | Pyridine | -8.86980 | -8.86960 |
| 14 | Pyrazine | -8.96430 | -8.96380 |
| 15 | Pyrimidine | -8.99290 | -8.99370 |
| 16 | Pyridazine | -8.42420 | -8.42460 |
| 17 | Triazine | -9.69700 | -9.69590 |
| 18 | Tetrazine | -9.05010 | -9.04860 |
| 19 | Formaldehyde | -10.15540 | -10.15600 |
| 20 | Acetone | -8.84510 | -8.84440 |
| 21 | Benzoquinone | -8.87530 | -8.87670 |
| 22 | Formamide | -9.24620 | -9.24640 |
| 23 | Acetamide | -8.83810 | -8.83810 |
| 24 | Propanamide | -8.74740 | -8.74740 |
| 25 | Cytosine | -8.03170 | -8.03150 |
| 26 | Thymine | -8.50020 | -8.49890 |
| 27 | Uracil | -8.96410 | -8.96390 |
| 28 | Adenine | -7.70740 | -7.70660 |

Table S9: Carbon clusters quasiparticle energies in eV

| | | RI-V | | | | RI-RS | | | |
|---|---|---|---|---|---|---|---|---|---|
| | | HOMO | | LUMO | | HOMO | | LUMO | |
| | atoms | spin ↑ | spin ↓ | spin ↑ | spin ↓ | spin ↑ | spin ↓ | spin ↑ | spin ↓ |
| 1 | 29 | -7.4590 | -7.2559 | -0.3703 | -0.1729 | -7.4600 | -7.2561 | -0.3702 | -0.1730 |
| 2 | 40 | -6.3532 | -6.7609 | -0.5826 | -0.3258 | -6.3532 | -6.7615 | -0.5829 | -0.3258 |
| 3 | 47 | -7.6150 | -6.8442 | -0.7405 | -0.8345 | -7.6151 | -6.8443 | -0.7407 | -0.8343 |
| 4 | 55 | -6.9806 | -6.8987 | -1.4363 | -0.7387 | -6.9809 | -6.8987 | -1.4366 | -0.7388 |
| 5 | 59 | -7.8332 | -7.8332 | 2.3369 | 2.3369 | -7.8345 | -7.8345 | 2.3370 | 2.3370 |
| 6 | 61 | -6.4373 | -7.1503 | -1.0461 | 0.0442 | -6.4365 | -7.1492 | -1.0463 | 0.0439 |
| 7 | 89 | -6.9285 | -6.9285 | 0.8755 | 0.8755 | -6.9286 | -6.9287 | 0.8756 | 0.8756 |
| 8 | 94 | -5.9211 | -5.7267 | 1.2080 | 0.6125 | -5.9210 | -5.7263 | 1.2080 | 0.6121 |
| 9 | 106 | -4.3628 | -5.8161 | 0.8115 | 0.7072 | -4.3627 | -5.8156 | 0.8114 | 0.7072 |
| 10 | 116 | -5.0193 | -5.7309 | 1.0382 | 1.1529 | -5.0189 | -5.7319 | 1.0376 | 1.1526 |

# S4 Total, atomization and quasiparticle energies employing the Def2-TZVP basis set

Table S10: Total Hartree-Fock energies in eV

| | Thiel set | no-RI | RI-V | RI-RS |
|---|---|---|---|---|
| 1 | Ethene | -2124.24577402 | -2124.24560566 | -2124.24774404 |
| 2 | Butadiene | -4217.20194931 | -4217.20199296 | -4217.20292315 |
| 3 | Hexatriene | -6310.16730005 | -6310.16603632 | -6310.16327477 |
| 4 | Octatetraene | -8403.13341300 | -8403.13329512 | -8403.13632604 |
| 5 | Cyclopropene | -3152.88941636 | -3152.88928640 | -3152.88759961 |
| 6 | Cyclopentadiene | -5247.99837696 | -5247.99921969 | -5247.99985875 |
| 7 | Norbornadiene | -7340.08675975 | -7340.08856530 | -7340.08337346 |
| 8 | Benzene | -6279.93099094 | -6279.93125591 | -6279.93320546 |
| 9 | Naphthalene | -10435.08286304 | -10435.08348031 | -10435.08667997 |
| 10 | Furan | -6223.57064934 | -6223.57051453 | -6223.56824350 |
| 11 | Pyrrole | -5684.11250405 | -5684.11292315 | -5684.10756287 |
| 12 | Imidazole | -6119.80507130 | -6119.80515179 | -6119.79841600 |
| 13 | Pyridine | -6715.25558275 | -6715.25606192 | -6715.26214545 |
| 14 | Pyrazine | -7150.42699036 | -7150.42628690 | -7150.42677219 |
| 15 | Pyrimidine | -7150.73639332 | -7150.73639660 | -7150.74115985 |
| 16 | Pyridazine | -7149.50345903 | -7149.50322955 | -7149.50234039 |
| 17 | Triazine | -7586.36515728 | -7586.36453385 | -7586.35744199 |
| 18 | Tetrazine | -8018.99871078 | -8018.99822673 | -8018.99472514 |
| 19 | Formaldehyde | -3099.76701967 | -3099.76699958 | -3099.76275829 |
| 20 | Acetone | -5225.59362514 | -5225.59285618 | -5225.58778893 |
| 21 | Benzoquinone | -10323.21875313 | -10323.21985265 | -10323.21051320 |
| 22 | Formamide | -4598.87202922 | -4598.87219146 | -4598.87168065 |
| 23 | Acetamide | -5661.70848078 | -5661.70784713 | -5661.70399764 |
| 24 | Propanamide | -6724.26603187 | -6724.26618851 | -6724.26503674 |
| 25 | Cytosine | -10687.80695579 | -10687.80657776 | -10687.80675166 |
| 26 | Thymine | -12290.88010399 | -12290.87956700 | -12290.87036806 |
| 27 | Uracil | -11228.23101579 | -11228.23079579 | -11228.23635827 |
| 28 | Adenine | -12644.84165674 | -12644.84174573 | -12644.84616546 |
| | Atom | | | |
| 1 | Hydrogen | -13.60051752 | -13.60051403 | -13.60051403 |
| 2 | Carbon | -1025.66453417 | -1025.66455241 | -1025.66502120 |
| 3 | Nitrogen | -1480.37406330 | -1480.37409655 | -1480.37365990 |
| 4 | Oxygen | -2035.83674083 | -2035.83681656 | -2035.83705158 |

Table S11: Hartree-Fock exchange energies in eV

| | Thiel set | no-RI | RI-V | RI-RS |
|---|---|---|---|---|
| 1 | Ethene | -319.51265228 | -319.51269704 | -319.51537529 |
| 2 | Butadiene | -620.88277954 | -620.88369255 | -620.88422442 |
| 3 | Hexatriene | -922.27009459 | -922.27154469 | -922.26661592 |
| 4 | Octatetraene | -1223.65298729 | -1223.65529810 | -1223.65898780 |
| 5 | Cyclopropene | -460.46548404 | -460.46579723 | -460.46445005 |
| 6 | Cyclopentadiene | -763.41400483 | -763.41625301 | -763.41675813 |
| 7 | Norbornadiene | -1066.27421557 | -1066.27785951 | -1066.27384795 |
| 8 | Benzene | -904.63389114 | -904.63649909 | -904.63834299 |
| 9 | Naphthalene | -1489.55050873 | -1489.55502189 | -1489.55972989 |
| 10 | Furan | -826.84364490 | -826.85005775 | -826.84827595 |
| 11 | Pyrrole | -792.89044613 | -792.89423911 | -792.88909638 |
| 12 | Imidazole | -821.66473282 | -821.66801110 | -821.66080602 |
| 13 | Pyridine | -933.30085593 | -933.30061957 | -933.30850069 |
| 14 | Pyrazine | -961.56218021 | -961.56339716 | -961.56530305 |
| 15 | Pyrimidine | -962.23226597 | -962.22844911 | -962.23626382 |
| 16 | Pyridazine | -960.49981736 | -960.49892315 | -960.49578127 |
| 17 | Triazine | -991.37265335 | -991.36924976 | -991.35970098 |
| 18 | Tetrazine | -1016.03660215 | -1016.03713088 | -1016.03731848 |
| 19 | Formaldehyde | -382.95740476 | -382.95579711 | -382.95194183 |
| 20 | Acetone | -705.41973367 | -705.41693751 | -705.41175295 |
| 21 | Benzoquinone | -1332.31476983 | -1332.31815113 | -1332.30702660 |
| 22 | Formamide | -574.14397925 | -574.14100016 | -574.13909847 |
| 23 | Acetamide | -735.39346522 | -735.39179419 | -735.38835633 |
| 24 | Propanamide | -896.54270721 | -896.54171180 | -896.54023488 |
| 25 | Cytosine | -1378.96616007 | -1378.97263343 | -1378.97005170 |
| 26 | Thymine | -1574.66179769 | -1574.66450288 | -1574.65425361 |
| 27 | Uracil | -1413.43580092 | -1413.43883041 | -1413.44222826 |
| 28 | Adenine | -1655.87703935 | -1655.88588662 | -1655.89169364 |
| | Atom | | | |
| 1 | Hydrogen | -8.50476287 | -8.50476467 | -8.50476467 |
| 2 | Carbon | -138.13941286 | -138.13944597 | -138.13989825 |
| 3 | Nitrogen | -179.77784730 | -179.77776348 | -179.77735422 |
| 4 | Oxygen | -223.62218760 | -223.62208256 | -223.62247675 |

Table S12: MP2 correlation energies in eV

| | Thiel set | no-RI | RI-V | RI-RS |
|---|---|---|---|---|
| 1 | Ethene | -9.78329420 | -9.78315941 | -9.78330472 |
| 2 | Butadiene | -19.18248904 | -19.18240972 | -19.18262197 |
| 3 | Hexatriene | -28.63354259 | -28.63348111 | -28.63372983 |
| 4 | Octatetraene | -38.10471910 | -38.10468077 | -38.10554637 |
| 5 | Cyclopropene | -14.42022424 | -14.42003837 | -14.41956408 |
| 6 | Cyclopentadiene | -23.94082470 | -23.94069336 | -23.94081255 |
| 7 | Norbornadiene | -33.95242545 | -33.95188009 | -33.95354461 |
| 8 | Benzene | -28.35140934 | -28.35153961 | -28.35196220 |
| 9 | Naphthalene | -47.05160447 | -47.05176577 | -47.05223435 |
| 10 | Furan | -25.82943930 | -25.82967094 | -25.82996047 |
| 11 | Pyrrole | -25.19408118 | -25.19412919 | -25.19457383 |
| 12 | Imidazole | -26.19105355 | -26.19115922 | -26.19182372 |
| 13 | Pyridine | -29.35073134 | -29.35095172 | -29.35157758 |
| 14 | Pyrazine | -30.41969531 | -30.42015885 | -30.42072485 |
| 15 | Pyrimidine | -30.26963273 | -30.26985187 | -30.26963391 |
| 16 | Pyridazine | -30.54660127 | -30.54705071 | -30.54715819 |
| 17 | Triazine | -31.11986272 | -31.12001661 | -31.12016546 |
| 18 | Tetrazine | -32.74239047 | -32.74313651 | -32.74247473 |
| 19 | Formaldehyde | -11.61101174 | -11.61098620 | -11.61147873 |
| 20 | Acetone | -21.69246490 | -21.69243381 | -21.69302022 |
| 21 | Benzoquinone | -41.12360836 | -41.12438172 | -41.12572705 |
| 22 | Formamide | -17.70433811 | -17.70427289 | -17.70419642 |
| 23 | Acetamide | -22.73197644 | -22.73196067 | -22.73259551 |
| 24 | Propanamide | -27.81642508 | -27.81641358 | -27.81682910 |
| 25 | Cytosine | -43.10155857 | -43.10183711 | -43.10151139 |
| 26 | Thymine | -48.96950048 | -48.96991776 | -48.97073818 |
| 27 | Uracil | -43.79673472 | -43.79708445 | -43.79716853 |
| 28 | Adenine | -52.78030440 | -52.78057337 | -52.78045337 |
| | Atom | | | |
| 1 | Hydrogen | 0.00000000 | 0.00000000 | 0.00000000 |
| 2 | Carbon | -2.23811478 | -2.23809447 | -2.23808359 |
| 3 | Nitrogen | -3.05112244 | -3.05108057 | -3.05109091 |
| 4 | Oxigen | -4.34134836 | -4.34129367 | -4.34126809 |

Table S13: Hartree-Fock and MP2 atomization energies in eV

| | | Hartree-Fock | | | MP2 | | |
|---|---|---|---|---|---|---|---|
| | Thiel set | no-RI | RI-V | RI-RS | no-RI | RI-V | RI-RS |
| 1 | Ethene | 18.51463560 | 18.51444474 | 18.51564554 | 23.82170023 | 23.82141521 | 23.82158229 |
| 2 | Butadiene | 32.94070750 | 32.94069917 | 32.93975420 | 43.17073742 | 43.17073101 | 43.17098680 |
| 3 | Hexatriene | 47.37595487 | 47.37460966 | 47.36903537 | 62.58080877 | 62.57952396 | 62.57983798 |
| 4 | Octatetraene | 61.81196443 | 61.81173560 | 61.81101620 | 82.01176528 | 82.01166061 | 82.01261328 |
| 5 | Cyclopropene | 21.49374377 | 21.49357307 | 21.49047991 | 29.19962367 | 29.19932804 | 29.19888640 |
| 6 | Cyclopentadiene | 38.07260099 | 38.07337350 | 38.07166860 | 50.82285178 | 50.82359451 | 50.82376812 |
| 7 | Norbornadiene | 51.63088039 | 51.63258623 | 51.62411286 | 69.91650237 | 69.91780504 | 69.91954575 |
| 8 | Benzene | 44.34068080 | 44.34085730 | 44.33999412 | 59.26340144 | 59.26383009 | 59.26431799 |
| 9 | Naphthalene | 69.63338118 | 69.63384402 | 69.63235578 | 94.30383783 | 94.30466509 | 94.30524252 |
| 10 | Furan | 30.67370175 | 30.67343223 | 30.66905102 | 43.20933356 | 43.20943162 | 43.20979027 |
| 11 | Pyrrole | 46.67823399 | 46.67856086 | 46.67176207 | 59.86873360 | 59.86923160 | 59.86970944 |
| 12 | Imidazole | 27.66127211 | 27.66124536 | 27.65397650 | 41.03573642 | 41.03596003 | 41.03663650 |
| 13 | Pyridine | 38.55626100 | 38.55663320 | 38.56080943 | 53.66529598 | 53.66603200 | 53.66670194 |
| 14 | Pyrazine | 32.61865700 | 32.61782805 | 32.61731149 | 47.98364829 | 47.98344789 | 47.98403674 |
| 15 | Pyrimidine | 32.92805996 | 32.92793775 | 32.93169915 | 48.14298867 | 48.14325061 | 48.14305550 |
| 16 | Pyridazine | 31.69512567 | 31.69477071 | 31.69287969 | 47.18702292 | 47.18728240 | 47.18741274 |
| 17 | Triazine | 27.44781231 | 27.44704489 | 27.43985661 | 42.69996335 | 42.69953639 | 42.69968687 |
| 18 | Tetrazine | 18.97235420 | 18.97170764 | 18.96901509 | 35.03402533 | 35.03433294 | 35.03365157 |
| 19 | Formaldehyde | 11.06470962 | 11.06460255 | 11.05965746 | 16.09625821 | 16.09620061 | 16.09672960 |
| 20 | Acetone | 31.16017667 | 31.15929823 | 31.15258959 | 41.79694886 | 41.79615497 | 41.79679960 |
| 21 | Benzoquinone | 43.15599636 | 43.15684897 | 43.14422674 | 62.16821930 | 62.17007653 | 62.17153832 |
| 22 | Formamide | 16.19513835 | 16.19518386 | 16.19440589 | 24.26889087 | 24.26898803 | 24.26893769 |
| 23 | Acetamide | 26.16602070 | 26.16525907 | 26.16067363 | 37.02929676 | 37.02865656 | 37.02932841 |
| 24 | Propanamide | 35.85800258 | 35.85801999 | 35.85566348 | 49.56761250 | 49.56777592 | 49.56823933 |
| 25 | Cytosine | 40.18730077 | 40.18669178 | 40.18606545 | 60.84168451 | 60.84161563 | 60.84132801 |
| 26 | Thymine | 48.53271975 | 48.53189457 | 48.52075495 | 71.52670470 | 71.52659150 | 71.52749682 |
| 27 | Uracil | 38.74920076 | 38.74870382 | 38.75279440 | 58.80853473 | 58.80866191 | 58.80882001 |
| 28 | Adenine | 46.64608179 | 46.64593079 | 46.65018983 | 72.98020005 | 72.98062898 | 72.98051169 |

Table S14: GW100 quasiparticle energies in eV

| | | RI-V | | RI-RS | |
|---|---|---|---|---|---|
| CAS | Formula | HOMO | LUMO | HOMO | LUMO |
| 7440-59-7 | He | -23.7709 | 22.2740 | -23.7709 | 22.2740 |
| 7440-01-9 | Ne | -20.7617 | 20.8807 | -20.7617 | 20.8808 |
| 7440-37-1 | Ar | -15.1981 | 14.7038 | -15.1974 | 14.7037 |
| 7439-90-9 | Kr | -13.5439 | 10.3977 | -13.5455 | 10.3979 |
| 1333-74-0 | $H_2$ | -15.9479 | 4.4617 | -15.9479 | 4.4617 |
| 14452-59-6 | $Li_2$ | -5.0418 | -0.1880 | -5.0402 | -0.1878 |
| 25681-79-2 | $Na_2$ | -4.9076 | -0.3646 | -4.9031 | -0.3654 |
| 39297-86-4 | $Na_4$ | -4.1682 | -0.7060 | -4.1652 | -0.7067 |
| 39297-88-6 | $Na_6$ | -4.2917 | -0.6805 | -4.2895 | -0.6806 |
| 25681-80-5 | $K_2$ | -3.9837 | -0.4386 | -3.9865 | -0.4391 |
| 7727-37-9 | $N_2$ | -15.2464 | 2.9051 | -15.2470 | 2.9052 |
| 12185-09-0 | $P_2$ | -10.1742 | -0.2716 | -10.1741 | -0.2717 |
| 23878-46-8 | $As_2$ | -9.4517 | -0.3563 | -9.4503 | -0.3567 |
| 7782-41-4 | $F_2$ | -15.3329 | 0.1378 | -15.3327 | 0.1379 |
| 7782-50-5 | $Cl_2$ | -11.1344 | -0.2001 | -11.1339 | -0.2006 |
| 7726-95-6 | $Br_2$ | -10.2128 | -0.8822 | -10.2111 | -0.8827 |
| 74-82-8 | $CH_4$ | -14.0446 | 3.5597 | -14.0445 | 3.5591 |
| 74-84-0 | $C_2H_6$ | -12.4448 | 3.1993 | -12.4453 | 3.1992 |
| 74-98-6 | $C_3H_8$ | -11.8721 | 3.0083 | -11.8723 | 3.0082 |
| 106-97-8 | $C_4H_{10}$ | -11.5723 | 2.9291 | -11.5723 | 2.9290 |
| 74-85-1 | $C_2H_4$ | -10.3473 | 2.5821 | -10.3475 | 2.5823 |
| 74-86-2 | $C_2H_2$ | -11.1193 | 3.4528 | -11.1191 | 3.4526 |
| 12184-80-4 | $C_4$ | -11.0134 | -2.5153 | -11.0132 | -2.5157 |
| 75-19-4 | $C_3H_6$ | -10.6149 | 3.5300 | -10.6146 | 3.5299 |
| 71-43-2 | $C_6H_6$ | -9.0149 | 1.5996 | -9.0152 | 1.5998 |
| 629-20-9 | $C_8H_8$ | -8.0895 | 0.5736 | -8.0894 | 0.5783 |
| 542-92-7 | $C_5H_6$ | -8.3690 | 1.5722 | -8.3691 | 1.5724 |
| 75-02-5 | $C_2H_3F$ | -10.2385 | 2.7238 | -10.2388 | 2.7241 |
| 75-01-4 | $C_2H_3Cl$ | -9.7899 | 2.0098 | -9.7893 | 2.0098 |
| 593-60-2 | $C_2H_3Br$ | -8.9740 | 1.9325 | -8.9741 | 1.9326 |
| 75-73-0 | $CF_4$ | -15.7430 | 4.9632 | -15.7423 | 4.9636 |
| 56-23-5 | $CCl_4$ | -11.1443 | 0.7778 | -11.1427 | 0.7779 |
| 558-13-4 | $CBr_4$ | -10.0340 | -0.5240 | -10.0326 | -0.5241 |
| 7803-62-5 | $SiH_4$ | -12.4647 | 3.2173 | -12.4645 | 3.2172 |
| 7782-65-2 | $GeH_4$ | -12.1560 | 3.3115 | -12.1555 | 3.3114 |
| 1590-87-0 | $Si_2H_6$ | -10.3485 | 2.2709 | -10.3483 | 2.2709 |
| 14868-53-2 | $Si_5H_{12}$ | -8.9810 | 0.7297 | -8.9808 | 0.7296 |
| 7580-67-8 | LiH | -7.3011 | 0.1781 | -7.3004 | 0.1781 |
| 7693-26-7 | KH | -5.4038 | 0.0443 | -5.4060 | 0.0442 |
| 13283-31-3 | $BH_3$ | -13.0069 | 0.4547 | -13.0067 | 0.4546 |
| 19287-45-7 | $B_2H_6$ | -11.9938 | 1.2447 | -11.9939 | 1.2447 |
| 7664-41-7 | $NH_3$ | -10.4843 | 3.0422 | -10.4841 | 3.0422 |
| 7782-79-8 | $HN_3$ | -10.4815 | 1.8778 | -10.4819 | 1.8779 |
| 7803-51-2 | $PH_3$ | -10.2788 | 3.1453 | -10.2787 | 3.1452 |
| 7784-42-1 | $AsH_3$ | -10.1328 | 3.0704 | -10.1324 | 3.0704 |
| 7783-06-4 | $SH_2$ | -10.0095 | 3.2381 | -10.0092 | 3.2380 |
| 7664-39-3 | FH | -15.5484 | 3.2698 | -15.5484 | 3.2698 |
| 7647-01-0 | ClH | -12.2655 | 2.8886 | -12.2654 | 2.8885 |
| 7789-24-4 | LiF | -10.4583 | 0.1220 | -10.4562 | 0.1220 |
| 7783-40-6 | $F_2Mg$ | -12.9907 | 0.0600 | -12.9904 | 0.0602 |
| 7783-63-3 | $TiF_4$ | -14.6657 | -0.2168 | -14.6658 | -0.2165 |
| 7784-18-1 | $AlF_3$ | -14.6977 | 0.6739 | -14.6978 | 0.6740 |
| 13768-60-0 | BF | -10.7673 | 1.5094 | -10.7677 | 1.5097 |
| 7783-60-0 | $SF_4$ | -12.2714 | 0.9831 | -12.2725 | 0.9830 |

(*Table S14 continues*)

(*Table S14 continued*)

| CAS | Formula | RI-V HOMO | RI-V LUMO | RI-RS HOMO | RI-RS LUMO |
|---|---|---|---|---|---|
| 7758-02-3 | BrK | -7.7204 | -0.2594 | -7.7205 | -0.2593 |
| 17108-85-9 | GaCl | -9.5424 | 0.3370 | -9.5440 | 0.3373 |
| 7647-14-5 | NaCl | -8.5718 | -0.4090 | -8.5721 | -0.4092 |
| 7786-30-3 | $MgCl_2$ | -11.2478 | -0.1141 | -11.2476 | -0.1141 |
| 10043-11-5 | BN | -11.3784 | -3.5955 | -11.3779 | -3.5956 |
| 74-90-8 | NCH | -13.3570 | 3.1555 | -13.3559 | 3.1554 |
| 17739-47-8 | PN | -11.5004 | 0.2863 | -11.5009 | 0.2863 |
| 302-01-2 | $H_2NNH_2$ | -9.4259 | 2.6681 | -9.4264 | 2.6681 |
| 50-00-0 | $H_2CO$ | -10.5445 | 1.5736 | -10.5439 | 1.5734 |
| 67-56-1 | $CH_4O$ | -10.7247 | 3.1636 | -10.7247 | 3.1634 |
| 64-17-5 | $C_2H_6O$ | -10.3570 | 2.9507 | -10.3565 | 2.9505 |
| 75-07-0 | $C_2H_4O$ | -9.8619 | 1.7294 | -9.8616 | 1.7296 |
| 60-29-7 | $C_4H_{10}O$ | -9.5333 | 3.0009 | -9.5327 | 3.0004 |
| 64-18-6 | $CH_2O_2$ | -11.0604 | 2.5914 | -11.0603 | 2.5911 |
| 7722-84-1 | HOOH | -11.2228 | 3.1780 | -11.2219 | 3.1781 |
| 7732-18-5 | $H_2O$ | -12.1647 | 3.0795 | -12.1646 | 3.0796 |
| 124-38-9 | $CO_2$ | -13.4375 | 2.9405 | -13.4375 | 2.9409 |
| 75-15-0 | $CS_2$ | -9.7576 | 0.2578 | -9.7576 | 0.2575 |
| 463-58-1 | OCS | -10.9466 | 1.7280 | -10.9466 | 1.7277 |
| 1603-84-5 | OCSe | -10.2042 | 1.3108 | -10.2047 | 1.3107 |
| 630-08-0 | CO | -13.9585 | 1.0785 | -13.9580 | 1.0786 |
| 10028-15-6 | $O_3$ | -12.3626 | -1.8647 | -12.3623 | -1.8648 |
| 7446-09-5 | $SO_2$ | -12.0066 | -0.4402 | -12.0057 | -0.4403 |
| 1304-56-9 | BeO | -9.4692 | -1.9943 | -9.4697 | -1.9941 |
| 1309-48-4 | MgO | -7.3194 | -1.5743 | -7.3193 | -1.5742 |
| 108-88-3 | $C_7H_8$ | -8.6323 | 1.5333 | -8.6320 | 1.5334 |
| 100-41-4 | $C_8H_{10}$ | -8.5809 | 1.5683 | -8.5810 | 1.5683 |
| 392-56-3 | $C_6F_6$ | -9.6568 | 0.9101 | -9.6563 | 0.9100 |
| 108-95-2 | $C_6H_5OH$ | -8.3970 | 1.4666 | -8.3967 | 1.4665 |
| 62-53-3 | $C_6H_5NH_2$ | -7.6941 | 1.6767 | -7.6943 | 1.6765 |
| 110-86-1 | $C_5H_5N$ | -9.3874 | 1.0332 | -9.3865 | 1.0331 |
| 73-40-5 | $C_5H_5N5O$ | -7.7440 | 1.3764 | -7.7439 | 1.3763 |
| 73-24-5 | $C_5H_5N_5O$ | -8.0273 | 1.0622 | -8.0272 | 1.0621 |
| 71-30-7 | $C_4H_5N_3O$ | -8.4546 | 0.8031 | -8.4550 | 0.8031 |
| 65-71-4 | $C_5H_6N_2O_2$ | -8.8335 | 0.5945 | -8.8334 | 0.5943 |
| 66-22-8 | $C_4H_4N_2O_2$ | -9.2338 | 0.5438 | -9.2338 | 0.5438 |
| 57-13-6 | $CH_4N_2O$ | -9.6616 | 2.4055 | -9.6612 | 2.4053 |
| 12190-70-4 | $Cu_2$ | -7.3312 | -0.3586 | -7.3308 | -0.3587 |
| 544-92-3 | NCCu | -10.0067 | -1.0312 | -10.0066 | -1.0312 |

## S5 Details of RI-RS workflow

The workflow of the computation of the different methods used in this work is explained in the algorithm 1. First, if the use of the Hartree-Fock method is requested, the flag `hartree_fock` is set to true, and the fitting coefficients $[M_{ij}^{\mu}]_{\text{RI-RS}}$ is calculated (step 2). Next, the SCF starts until the convergence is reached. Regardless of the method required in every SCF iteration, the Roothaan-Hall equations are solved to obtain the orbital energies and molecular orbital (MO) coefficients. For Hartree-Fock, the Fock exchange energy, $E^{\text{HF}}$ is calculated, Equation (40) in the manuscript.

If post-SCF energy corrections are requested. We verify if the fitting coefficients are already calculated, i.e `hartree_fock` is set to true. Also requested in MP2 and CCSD methods. If `hartree_fock` flag is false, namely, a DFT calculation was requested. Therefore, the fitting coefficients are calculated in step 13. Next, we obtain the $\varepsilon_n$ energies and MO coefficients from the SCF. Following by the transformation of fitting coefficients into their MO representation, $[O_{mn}^{\mu}]_{\text{RI-RS}}$. Finally, the post-SCF calculations continue.

**Algorithm 1:** Computation of Hartree-Fock and post-SCF energy corrections using the separable resolution of the identity approach

1 **if** *Hartree-Fock is requested* **then**<br>
2     `hartree_fock` = .TRUE.<br>
3     Calculate $[M_{ij}^{\mu}]_{\text{RI-RS}}$<br>
4 **end if**<br>
5 **repeat**<br>
6     Get $\{\varepsilon_n\}$ and $c_{mi}$ from previous iteration<br>
7     **if** `hartree_fock` **then**<br>
8         Calculate $E_x^F$ from $[O_{mn}^{\mu}]_{\text{RI-RS}}$<br>
9     **end if**<br>
10 **until** *SCF is converged*<br>
11 **if** *post-SCF correction are requested* **then**<br>
12     **if** `.NOT.hartree_fock` **then**<br>
13         Calculate $[M_{ij}^{\mu}]_{\text{RI-RS}}$<br>
14     **end if**<br>
15     Get $\{\varepsilon_n\}$ and $c_{mi}$ from the SCF<br>
16     Calculate $[O_{mn}^{\mu}]_{\text{RI-RS}}$ using Eq.<br>
17     Continue post-SCF corrections<br>
18 **end if**
